# Supplementary material for: Multigrid Neural Architectures
Source: arXiv:1611.07661 source file (2017-05-11)
Supplement: Supplementary file 1 [file fig_supp_seg_content.tex]

\setlength\fboxsep{0pt}
\begin{minipage}[t]{0.4975\linewidth}
   \vspace{0pt}
   % example 00156
   \begin{center}
   \begin{minipage}[t]{0.09\linewidth}
      \vspace{0pt}
      \begin{center}
         \tiny{\textbf{\textsf{Input}}}\\
         \fbox{\includegraphics[width=1.0\linewidth]{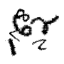}}
      \end{center}
   \end{minipage}
   \hfill
   \begin{minipage}[t]{0.90\linewidth}
      \vspace{0pt}
      \begin{center}
         % digits output
         \begin{minipage}[t]{0.94\linewidth}
            \vspace{0pt}
            \begin{center}
            \begin{minipage}[t]{0.09\linewidth}
               \vspace{0pt}
               \begin{center}
               \tiny{\textbf{\textsf{Digit: 0}}}\\
               \fbox{\includegraphics[width=1.0\linewidth]{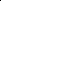}}
               \fbox{\includegraphics[width=1.0\linewidth]{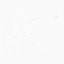}}
               \fbox{\includegraphics[width=1.0\linewidth]{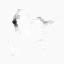}}
               \fbox{\includegraphics[width=1.0\linewidth]{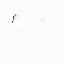}}
               \fbox{\includegraphics[width=1.0\linewidth]{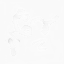}}
               \fbox{\includegraphics[width=1.0\linewidth]{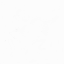}}
               \end{center}
            \end{minipage}
            \begin{minipage}[t]{0.09\linewidth}
               \vspace{0pt}
               \begin{center}
               \tiny{\textbf{\textsf{\phantom{g}1\phantom{g}}}}\\
               \fbox{\includegraphics[width=1.0\linewidth]{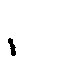}}
               \fbox{\includegraphics[width=1.0\linewidth]{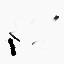}}
               \fbox{\includegraphics[width=1.0\linewidth]{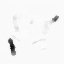}}
               \fbox{\includegraphics[width=1.0\linewidth]{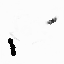}}
               \fbox{\includegraphics[width=1.0\linewidth]{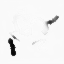}}
               \fbox{\includegraphics[width=1.0\linewidth]{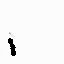}}
               \end{center}
            \end{minipage}
            \begin{minipage}[t]{0.09\linewidth}
               \vspace{0pt}
               \begin{center}
               \tiny{\textbf{\textsf{\phantom{g}2\phantom{g}}}}\\
               \fbox{\includegraphics[width=1.0\linewidth]{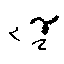}}
               \fbox{\includegraphics[width=1.0\linewidth]{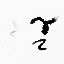}}
               \fbox{\includegraphics[width=1.0\linewidth]{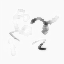}}
               \fbox{\includegraphics[width=1.0\linewidth]{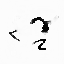}}
               \fbox{\includegraphics[width=1.0\linewidth]{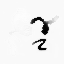}}
               \fbox{\includegraphics[width=1.0\linewidth]{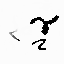}}
               \end{center}
            \end{minipage}
            \begin{minipage}[t]{0.09\linewidth}
               \vspace{0pt}
               \begin{center}
               \tiny{\textbf{\textsf{\phantom{g}3\phantom{g}}}}\\
               \fbox{\includegraphics[width=1.0\linewidth]{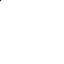}}
               \fbox{\includegraphics[width=1.0\linewidth]{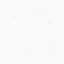}}
               \fbox{\includegraphics[width=1.0\linewidth]{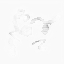}}
               \fbox{\includegraphics[width=1.0\linewidth]{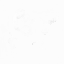}}
               \fbox{\includegraphics[width=1.0\linewidth]{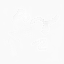}}
               \fbox{\includegraphics[width=1.0\linewidth]{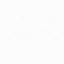}}
               \end{center}
            \end{minipage}
            \begin{minipage}[t]{0.09\linewidth}
               \vspace{0pt}
               \begin{center}
               \tiny{\textbf{\textsf{\phantom{g}4\phantom{g}}}}\\
               \fbox{\includegraphics[width=1.0\linewidth]{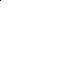}}
               \fbox{\includegraphics[width=1.0\linewidth]{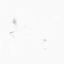}}
               \fbox{\includegraphics[width=1.0\linewidth]{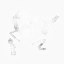}}
               \fbox{\includegraphics[width=1.0\linewidth]{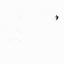}}
               \fbox{\includegraphics[width=1.0\linewidth]{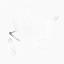}}
               \fbox{\includegraphics[width=1.0\linewidth]{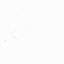}}
               \end{center}
            \end{minipage}
            \begin{minipage}[t]{0.09\linewidth}
               \vspace{0pt}
               \begin{center}
               \tiny{\textbf{\textsf{\phantom{g}5\phantom{g}}}}\\
               \fbox{\includegraphics[width=1.0\linewidth]{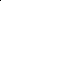}}
               \fbox{\includegraphics[width=1.0\linewidth]{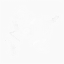}}
               \fbox{\includegraphics[width=1.0\linewidth]{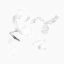}}
               \fbox{\includegraphics[width=1.0\linewidth]{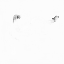}}
               \fbox{\includegraphics[width=1.0\linewidth]{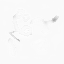}}
               \fbox{\includegraphics[width=1.0\linewidth]{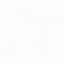}}
               \end{center}
            \end{minipage}
            \begin{minipage}[t]{0.09\linewidth}
               \vspace{0pt}
               \begin{center}
               \tiny{\textbf{\textsf{\phantom{g}6\phantom{g}}}}\\
               \fbox{\includegraphics[width=1.0\linewidth]{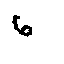}}
               \fbox{\includegraphics[width=1.0\linewidth]{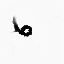}}
               \fbox{\includegraphics[width=1.0\linewidth]{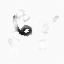}}
               \fbox{\includegraphics[width=1.0\linewidth]{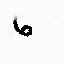}}
               \fbox{\includegraphics[width=1.0\linewidth]{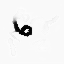}}
               \fbox{\includegraphics[width=1.0\linewidth]{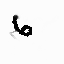}}
               \end{center}
            \end{minipage}
            \begin{minipage}[t]{0.09\linewidth}
               \vspace{0pt}
               \begin{center}
               \tiny{\textbf{\textsf{\phantom{g}7\phantom{g}}}}\\
               \fbox{\includegraphics[width=1.0\linewidth]{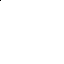}}
               \fbox{\includegraphics[width=1.0\linewidth]{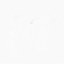}}
               \fbox{\includegraphics[width=1.0\linewidth]{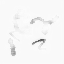}}
               \fbox{\includegraphics[width=1.0\linewidth]{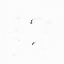}}
               \fbox{\includegraphics[width=1.0\linewidth]{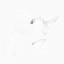}}
               \fbox{\includegraphics[width=1.0\linewidth]{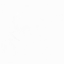}}
               \end{center}
            \end{minipage}
            \begin{minipage}[t]{0.09\linewidth}
               \vspace{0pt}
               \begin{center}
               \tiny{\textbf{\textsf{\phantom{g}8\phantom{g}}}}\\
               \fbox{\includegraphics[width=1.0\linewidth]{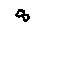}}
               \fbox{\includegraphics[width=1.0\linewidth]{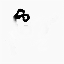}}
               \fbox{\includegraphics[width=1.0\linewidth]{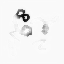}}
               \fbox{\includegraphics[width=1.0\linewidth]{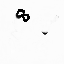}}
               \fbox{\includegraphics[width=1.0\linewidth]{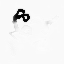}}
               \fbox{\includegraphics[width=1.0\linewidth]{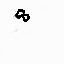}}
               \end{center}
            \end{minipage}
            \begin{minipage}[t]{0.09\linewidth}
               \vspace{0pt}
               \begin{center}
               \tiny{\textbf{\textsf{\phantom{g}9\phantom{g}}}}\\
               \fbox{\includegraphics[width=1.0\linewidth]{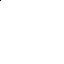}}
               \fbox{\includegraphics[width=1.0\linewidth]{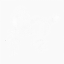}}
               \fbox{\includegraphics[width=1.0\linewidth]{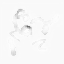}}
               \fbox{\includegraphics[width=1.0\linewidth]{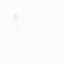}}
               \fbox{\includegraphics[width=1.0\linewidth]{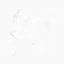}}
               \fbox{\includegraphics[width=1.0\linewidth]{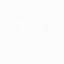}}
               \end{center}
            \end{minipage}
            \end{center}
         \end{minipage}
         % method labels
         \begin{minipage}[t]{0.04\linewidth}
            \vspace{0pt}
            \begin{rotate}{270}
               \tiny{\textbf{\textsf{
                  \hspace*{8pt}
                  True
                  \hspace*{4pt}
                  U-NET
                  \hspace*{7pt}
                  SG
                  \hspace*{8pt}
                  R-SG
                  \hspace*{6pt}
                  PMG
                  \hspace*{4pt}
                  R-PMG
               }}}
            \end{rotate}
         \end{minipage}
      \end{center}
   \end{minipage}
   \end{center}
\end{minipage}
\hfill
\begin{minipage}[t]{0.4975\linewidth}
   \vspace{0pt}
   % example 00170
   \begin{center}
   \begin{minipage}[t]{0.09\linewidth}
      \vspace{0pt}
      \begin{center}
         \tiny{\textbf{\textsf{Input}}}\\
         \fbox{\includegraphics[width=1.0\linewidth]{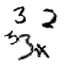}}
      \end{center}
   \end{minipage}
   \hfill
   \begin{minipage}[t]{0.90\linewidth}
      \vspace{0pt}
      \begin{center}
         % digits output
         \begin{minipage}[t]{0.94\linewidth}
            \vspace{0pt}
            \begin{center}
            \begin{minipage}[t]{0.09\linewidth}
               \vspace{0pt}
               \begin{center}
               \tiny{\textbf{\textsf{Digit: 0}}}\\
               \fbox{\includegraphics[width=1.0\linewidth]{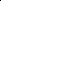}}
               \fbox{\includegraphics[width=1.0\linewidth]{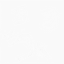}}
               \fbox{\includegraphics[width=1.0\linewidth]{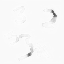}}
               \fbox{\includegraphics[width=1.0\linewidth]{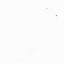}}
               \fbox{\includegraphics[width=1.0\linewidth]{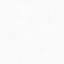}}
               \fbox{\includegraphics[width=1.0\linewidth]{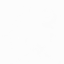}}
               \end{center}
            \end{minipage}
            \begin{minipage}[t]{0.09\linewidth}
               \vspace{0pt}
               \begin{center}
               \tiny{\textbf{\textsf{\phantom{g}1\phantom{g}}}}\\
               \fbox{\includegraphics[width=1.0\linewidth]{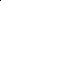}}
               \fbox{\includegraphics[width=1.0\linewidth]{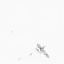}}
               \fbox{\includegraphics[width=1.0\linewidth]{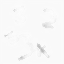}}
               \fbox{\includegraphics[width=1.0\linewidth]{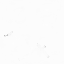}}
               \fbox{\includegraphics[width=1.0\linewidth]{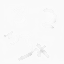}}
               \fbox{\includegraphics[width=1.0\linewidth]{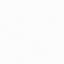}}
               \end{center}
            \end{minipage}
            \begin{minipage}[t]{0.09\linewidth}
               \vspace{0pt}
               \begin{center}
               \tiny{\textbf{\textsf{\phantom{g}2\phantom{g}}}}\\
               \fbox{\includegraphics[width=1.0\linewidth]{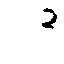}}
               \fbox{\includegraphics[width=1.0\linewidth]{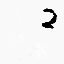}}
               \fbox{\includegraphics[width=1.0\linewidth]{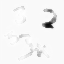}}
               \fbox{\includegraphics[width=1.0\linewidth]{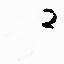}}
               \fbox{\includegraphics[width=1.0\linewidth]{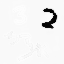}}
               \fbox{\includegraphics[width=1.0\linewidth]{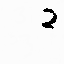}}
               \end{center}
            \end{minipage}
            \begin{minipage}[t]{0.09\linewidth}
               \vspace{0pt}
               \begin{center}
               \tiny{\textbf{\textsf{\phantom{g}3\phantom{g}}}}\\
               \fbox{\includegraphics[width=1.0\linewidth]{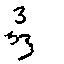}}
               \fbox{\includegraphics[width=1.0\linewidth]{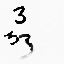}}
               \fbox{\includegraphics[width=1.0\linewidth]{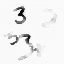}}
               \fbox{\includegraphics[width=1.0\linewidth]{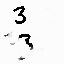}}
               \fbox{\includegraphics[width=1.0\linewidth]{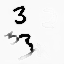}}
               \fbox{\includegraphics[width=1.0\linewidth]{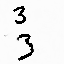}}
               \end{center}
            \end{minipage}
            \begin{minipage}[t]{0.09\linewidth}
               \vspace{0pt}
               \begin{center}
               \tiny{\textbf{\textsf{\phantom{g}4\phantom{g}}}}\\
               \fbox{\includegraphics[width=1.0\linewidth]{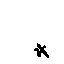}}
               \fbox{\includegraphics[width=1.0\linewidth]{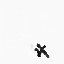}}
               \fbox{\includegraphics[width=1.0\linewidth]{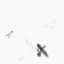}}
               \fbox{\includegraphics[width=1.0\linewidth]{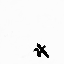}}
               \fbox{\includegraphics[width=1.0\linewidth]{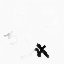}}
               \fbox{\includegraphics[width=1.0\linewidth]{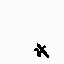}}
               \end{center}
            \end{minipage}
            \begin{minipage}[t]{0.09\linewidth}
               \vspace{0pt}
               \begin{center}
               \tiny{\textbf{\textsf{\phantom{g}5\phantom{g}}}}\\
               \fbox{\includegraphics[width=1.0\linewidth]{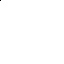}}
               \fbox{\includegraphics[width=1.0\linewidth]{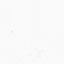}}
               \fbox{\includegraphics[width=1.0\linewidth]{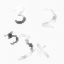}}
               \fbox{\includegraphics[width=1.0\linewidth]{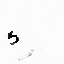}}
               \fbox{\includegraphics[width=1.0\linewidth]{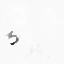}}
               \fbox{\includegraphics[width=1.0\linewidth]{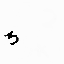}}
               \end{center}
            \end{minipage}
            \begin{minipage}[t]{0.09\linewidth}
               \vspace{0pt}
               \begin{center}
               \tiny{\textbf{\textsf{\phantom{g}6\phantom{g}}}}\\
               \fbox{\includegraphics[width=1.0\linewidth]{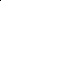}}
               \fbox{\includegraphics[width=1.0\linewidth]{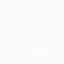}}
               \fbox{\includegraphics[width=1.0\linewidth]{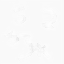}}
               \fbox{\includegraphics[width=1.0\linewidth]{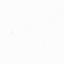}}
               \fbox{\includegraphics[width=1.0\linewidth]{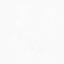}}
               \fbox{\includegraphics[width=1.0\linewidth]{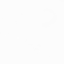}}
               \end{center}
            \end{minipage}
            \begin{minipage}[t]{0.09\linewidth}
               \vspace{0pt}
               \begin{center}
               \tiny{\textbf{\textsf{\phantom{g}7\phantom{g}}}}\\
               \fbox{\includegraphics[width=1.0\linewidth]{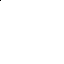}}
               \fbox{\includegraphics[width=1.0\linewidth]{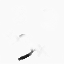}}
               \fbox{\includegraphics[width=1.0\linewidth]{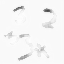}}
               \fbox{\includegraphics[width=1.0\linewidth]{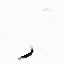}}
               \fbox{\includegraphics[width=1.0\linewidth]{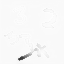}}
               \fbox{\includegraphics[width=1.0\linewidth]{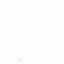}}
               \end{center}
            \end{minipage}
            \begin{minipage}[t]{0.09\linewidth}
               \vspace{0pt}
               \begin{center}
               \tiny{\textbf{\textsf{\phantom{g}8\phantom{g}}}}\\
               \fbox{\includegraphics[width=1.0\linewidth]{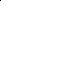}}
               \fbox{\includegraphics[width=1.0\linewidth]{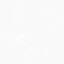}}
               \fbox{\includegraphics[width=1.0\linewidth]{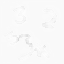}}
               \fbox{\includegraphics[width=1.0\linewidth]{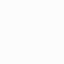}}
               \fbox{\includegraphics[width=1.0\linewidth]{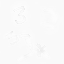}}
               \fbox{\includegraphics[width=1.0\linewidth]{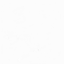}}
               \end{center}
            \end{minipage}
            \begin{minipage}[t]{0.09\linewidth}
               \vspace{0pt}
               \begin{center}
               \tiny{\textbf{\textsf{\phantom{g}9\phantom{g}}}}\\
               \fbox{\includegraphics[width=1.0\linewidth]{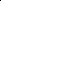}}
               \fbox{\includegraphics[width=1.0\linewidth]{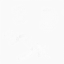}}
               \fbox{\includegraphics[width=1.0\linewidth]{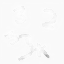}}
               \fbox{\includegraphics[width=1.0\linewidth]{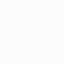}}
               \fbox{\includegraphics[width=1.0\linewidth]{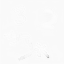}}
               \fbox{\includegraphics[width=1.0\linewidth]{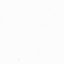}}
               \end{center}
            \end{minipage}
            \end{center}
         \end{minipage}
         % method labels
         \begin{minipage}[t]{0.04\linewidth}
            \vspace{0pt}
            \begin{rotate}{270}
               \tiny{\textbf{\textsf{
                  \hspace*{8pt}
                  True
                  \hspace*{4pt}
                  U-NET
                  \hspace*{7pt}
                  SG
                  \hspace*{8pt}
                  R-SG
                  \hspace*{6pt}
                  PMG
                  \hspace*{4pt}
                  R-PMG
               }}}
            \end{rotate}
         \end{minipage}
      \end{center}
   \end{minipage}
   \end{center}
\end{minipage}\\
\vspace{0.05\linewidth}
\begin{minipage}[t]{0.4975\linewidth}
   \vspace{0pt}
   % example 00171
   \begin{center}
   \begin{minipage}[t]{0.09\linewidth}
      \vspace{0pt}
      \begin{center}
         \tiny{\textbf{\textsf{Input}}}\\
         \fbox{\includegraphics[width=1.0\linewidth]{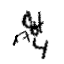}}
      \end{center}
   \end{minipage}
   \hfill
   \begin{minipage}[t]{0.90\linewidth}
      \vspace{0pt}
      \begin{center}
         % digits output
         \begin{minipage}[t]{0.94\linewidth}
            \vspace{0pt}
            \begin{center}
            \begin{minipage}[t]{0.09\linewidth}
               \vspace{0pt}
               \begin{center}
               \tiny{\textbf{\textsf{Digit: 0}}}\\
               \fbox{\includegraphics[width=1.0\linewidth]{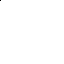}}
               \fbox{\includegraphics[width=1.0\linewidth]{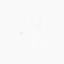}}
               \fbox{\includegraphics[width=1.0\linewidth]{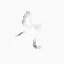}}
               \fbox{\includegraphics[width=1.0\linewidth]{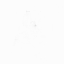}}
               \fbox{\includegraphics[width=1.0\linewidth]{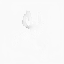}}
               \fbox{\includegraphics[width=1.0\linewidth]{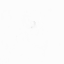}}
               \end{center}
            \end{minipage}
            \begin{minipage}[t]{0.09\linewidth}
               \vspace{0pt}
               \begin{center}
               \tiny{\textbf{\textsf{\phantom{g}1\phantom{g}}}}\\
               \fbox{\includegraphics[width=1.0\linewidth]{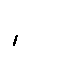}}
               \fbox{\includegraphics[width=1.0\linewidth]{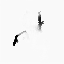}}
               \fbox{\includegraphics[width=1.0\linewidth]{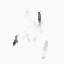}}
               \fbox{\includegraphics[width=1.0\linewidth]{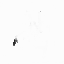}}
               \fbox{\includegraphics[width=1.0\linewidth]{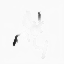}}
               \fbox{\includegraphics[width=1.0\linewidth]{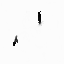}}
               \end{center}
            \end{minipage}
            \begin{minipage}[t]{0.09\linewidth}
               \vspace{0pt}
               \begin{center}
               \tiny{\textbf{\textsf{\phantom{g}2\phantom{g}}}}\\
               \fbox{\includegraphics[width=1.0\linewidth]{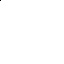}}
               \fbox{\includegraphics[width=1.0\linewidth]{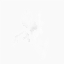}}
               \fbox{\includegraphics[width=1.0\linewidth]{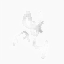}}
               \fbox{\includegraphics[width=1.0\linewidth]{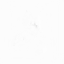}}
               \fbox{\includegraphics[width=1.0\linewidth]{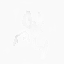}}
               \fbox{\includegraphics[width=1.0\linewidth]{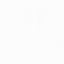}}
               \end{center}
            \end{minipage}
            \begin{minipage}[t]{0.09\linewidth}
               \vspace{0pt}
               \begin{center}
               \tiny{\textbf{\textsf{\phantom{g}3\phantom{g}}}}\\
               \fbox{\includegraphics[width=1.0\linewidth]{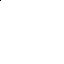}}
               \fbox{\includegraphics[width=1.0\linewidth]{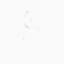}}
               \fbox{\includegraphics[width=1.0\linewidth]{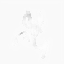}}
               \fbox{\includegraphics[width=1.0\linewidth]{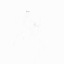}}
               \fbox{\includegraphics[width=1.0\linewidth]{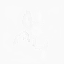}}
               \fbox{\includegraphics[width=1.0\linewidth]{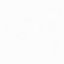}}
               \end{center}
            \end{minipage}
            \begin{minipage}[t]{0.09\linewidth}
               \vspace{0pt}
               \begin{center}
               \tiny{\textbf{\textsf{\phantom{g}4\phantom{g}}}}\\
               \fbox{\includegraphics[width=1.0\linewidth]{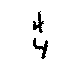}}
               \fbox{\includegraphics[width=1.0\linewidth]{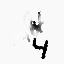}}
               \fbox{\includegraphics[width=1.0\linewidth]{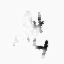}}
               \fbox{\includegraphics[width=1.0\linewidth]{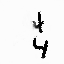}}
               \fbox{\includegraphics[width=1.0\linewidth]{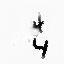}}
               \fbox{\includegraphics[width=1.0\linewidth]{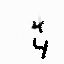}}
               \end{center}
            \end{minipage}
            \begin{minipage}[t]{0.09\linewidth}
               \vspace{0pt}
               \begin{center}
               \tiny{\textbf{\textsf{\phantom{g}5\phantom{g}}}}\\
               \fbox{\includegraphics[width=1.0\linewidth]{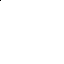}}
               \fbox{\includegraphics[width=1.0\linewidth]{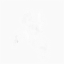}}
               \fbox{\includegraphics[width=1.0\linewidth]{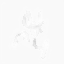}}
               \fbox{\includegraphics[width=1.0\linewidth]{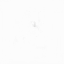}}
               \fbox{\includegraphics[width=1.0\linewidth]{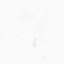}}
               \fbox{\includegraphics[width=1.0\linewidth]{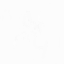}}
               \end{center}
            \end{minipage}
            \begin{minipage}[t]{0.09\linewidth}
               \vspace{0pt}
               \begin{center}
               \tiny{\textbf{\textsf{\phantom{g}6\phantom{g}}}}\\
               \fbox{\includegraphics[width=1.0\linewidth]{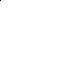}}
               \fbox{\includegraphics[width=1.0\linewidth]{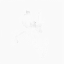}}
               \fbox{\includegraphics[width=1.0\linewidth]{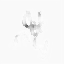}}
               \fbox{\includegraphics[width=1.0\linewidth]{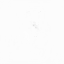}}
               \fbox{\includegraphics[width=1.0\linewidth]{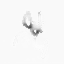}}
               \fbox{\includegraphics[width=1.0\linewidth]{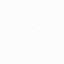}}
               \end{center}
            \end{minipage}
            \begin{minipage}[t]{0.09\linewidth}
               \vspace{0pt}
               \begin{center}
               \tiny{\textbf{\textsf{\phantom{g}7\phantom{g}}}}\\
               \fbox{\includegraphics[width=1.0\linewidth]{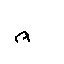}}
               \fbox{\includegraphics[width=1.0\linewidth]{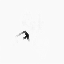}}
               \fbox{\includegraphics[width=1.0\linewidth]{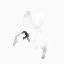}}
               \fbox{\includegraphics[width=1.0\linewidth]{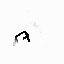}}
               \fbox{\includegraphics[width=1.0\linewidth]{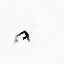}}
               \fbox{\includegraphics[width=1.0\linewidth]{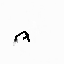}}
               \end{center}
            \end{minipage}
            \begin{minipage}[t]{0.09\linewidth}
               \vspace{0pt}
               \begin{center}
               \tiny{\textbf{\textsf{\phantom{g}8\phantom{g}}}}\\
               \fbox{\includegraphics[width=1.0\linewidth]{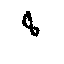}}
               \fbox{\includegraphics[width=1.0\linewidth]{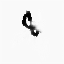}}
               \fbox{\includegraphics[width=1.0\linewidth]{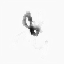}}
               \fbox{\includegraphics[width=1.0\linewidth]{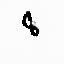}}
               \fbox{\includegraphics[width=1.0\linewidth]{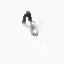}}
               \fbox{\includegraphics[width=1.0\linewidth]{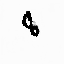}}
               \end{center}
            \end{minipage}
            \begin{minipage}[t]{0.09\linewidth}
               \vspace{0pt}
               \begin{center}
               \tiny{\textbf{\textsf{\phantom{g}9\phantom{g}}}}\\
               \fbox{\includegraphics[width=1.0\linewidth]{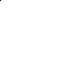}}
               \fbox{\includegraphics[width=1.0\linewidth]{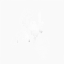}}
               \fbox{\includegraphics[width=1.0\linewidth]{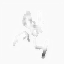}}
               \fbox{\includegraphics[width=1.0\linewidth]{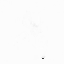}}
               \fbox{\includegraphics[width=1.0\linewidth]{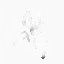}}
               \fbox{\includegraphics[width=1.0\linewidth]{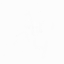}}
               \end{center}
            \end{minipage}
            \end{center}
         \end{minipage}
         % method labels
         \begin{minipage}[t]{0.04\linewidth}
            \vspace{0pt}
            \begin{rotate}{270}
               \tiny{\textbf{\textsf{
                  \hspace*{8pt}
                  True
                  \hspace*{4pt}
                  U-NET
                  \hspace*{7pt}
                  SG
                  \hspace*{8pt}
                  R-SG
                  \hspace*{6pt}
                  PMG
                  \hspace*{4pt}
                  R-PMG
               }}}
            \end{rotate}
         \end{minipage}
      \end{center}
   \end{minipage}
   \end{center}
\end{minipage}
\hfill
\begin{minipage}[t]{0.4975\linewidth}
   \vspace{0pt}
   % example 00200
   \begin{center}
   \begin{minipage}[t]{0.09\linewidth}
      \vspace{0pt}
      \begin{center}
         \tiny{\textbf{\textsf{Input}}}\\
         \fbox{\includegraphics[width=1.0\linewidth]{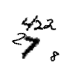}}
      \end{center}
   \end{minipage}
   \hfill
   \begin{minipage}[t]{0.90\linewidth}
      \vspace{0pt}
      \begin{center}
         % digits output
         \begin{minipage}[t]{0.94\linewidth}
            \vspace{0pt}
            \begin{center}
            \begin{minipage}[t]{0.09\linewidth}
               \vspace{0pt}
               \begin{center}
               \tiny{\textbf{\textsf{Digit: 0}}}\\
               \fbox{\includegraphics[width=1.0\linewidth]{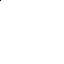}}
               \fbox{\includegraphics[width=1.0\linewidth]{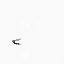}}
               \fbox{\includegraphics[width=1.0\linewidth]{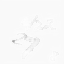}}
               \fbox{\includegraphics[width=1.0\linewidth]{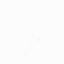}}
               \fbox{\includegraphics[width=1.0\linewidth]{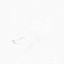}}
               \fbox{\includegraphics[width=1.0\linewidth]{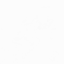}}
               \end{center}
            \end{minipage}
            \begin{minipage}[t]{0.09\linewidth}
               \vspace{0pt}
               \begin{center}
               \tiny{\textbf{\textsf{\phantom{g}1\phantom{g}}}}\\
               \fbox{\includegraphics[width=1.0\linewidth]{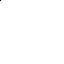}}
               \fbox{\includegraphics[width=1.0\linewidth]{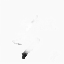}}
               \fbox{\includegraphics[width=1.0\linewidth]{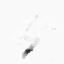}}
               \fbox{\includegraphics[width=1.0\linewidth]{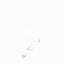}}
               \fbox{\includegraphics[width=1.0\linewidth]{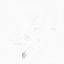}}
               \fbox{\includegraphics[width=1.0\linewidth]{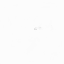}}
               \end{center}
            \end{minipage}
            \begin{minipage}[t]{0.09\linewidth}
               \vspace{0pt}
               \begin{center}
               \tiny{\textbf{\textsf{\phantom{g}2\phantom{g}}}}\\
               \fbox{\includegraphics[width=1.0\linewidth]{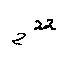}}
               \fbox{\includegraphics[width=1.0\linewidth]{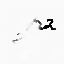}}
               \fbox{\includegraphics[width=1.0\linewidth]{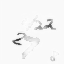}}
               \fbox{\includegraphics[width=1.0\linewidth]{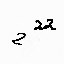}}
               \fbox{\includegraphics[width=1.0\linewidth]{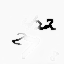}}
               \fbox{\includegraphics[width=1.0\linewidth]{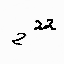}}
               \end{center}
            \end{minipage}
            \begin{minipage}[t]{0.09\linewidth}
               \vspace{0pt}
               \begin{center}
               \tiny{\textbf{\textsf{\phantom{g}3\phantom{g}}}}\\
               \fbox{\includegraphics[width=1.0\linewidth]{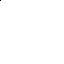}}
               \fbox{\includegraphics[width=1.0\linewidth]{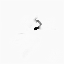}}
               \fbox{\includegraphics[width=1.0\linewidth]{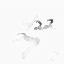}}
               \fbox{\includegraphics[width=1.0\linewidth]{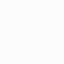}}
               \fbox{\includegraphics[width=1.0\linewidth]{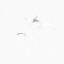}}
               \fbox{\includegraphics[width=1.0\linewidth]{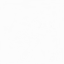}}
               \end{center}
            \end{minipage}
            \begin{minipage}[t]{0.09\linewidth}
               \vspace{0pt}
               \begin{center}
               \tiny{\textbf{\textsf{\phantom{g}4\phantom{g}}}}\\
               \fbox{\includegraphics[width=1.0\linewidth]{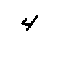}}
               \fbox{\includegraphics[width=1.0\linewidth]{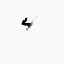}}
               \fbox{\includegraphics[width=1.0\linewidth]{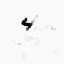}}
               \fbox{\includegraphics[width=1.0\linewidth]{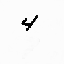}}
               \fbox{\includegraphics[width=1.0\linewidth]{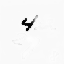}}
               \fbox{\includegraphics[width=1.0\linewidth]{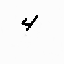}}
               \end{center}
            \end{minipage}
            \begin{minipage}[t]{0.09\linewidth}
               \vspace{0pt}
               \begin{center}
               \tiny{\textbf{\textsf{\phantom{g}5\phantom{g}}}}\\
               \fbox{\includegraphics[width=1.0\linewidth]{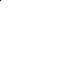}}
               \fbox{\includegraphics[width=1.0\linewidth]{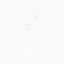}}
               \fbox{\includegraphics[width=1.0\linewidth]{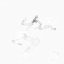}}
               \fbox{\includegraphics[width=1.0\linewidth]{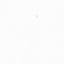}}
               \fbox{\includegraphics[width=1.0\linewidth]{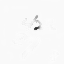}}
               \fbox{\includegraphics[width=1.0\linewidth]{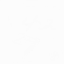}}
               \end{center}
            \end{minipage}
            \begin{minipage}[t]{0.09\linewidth}
               \vspace{0pt}
               \begin{center}
               \tiny{\textbf{\textsf{\phantom{g}6\phantom{g}}}}\\
               \fbox{\includegraphics[width=1.0\linewidth]{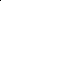}}
               \fbox{\includegraphics[width=1.0\linewidth]{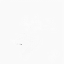}}
               \fbox{\includegraphics[width=1.0\linewidth]{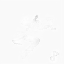}}
               \fbox{\includegraphics[width=1.0\linewidth]{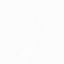}}
               \fbox{\includegraphics[width=1.0\linewidth]{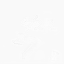}}
               \fbox{\includegraphics[width=1.0\linewidth]{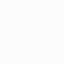}}
               \end{center}
            \end{minipage}
            \begin{minipage}[t]{0.09\linewidth}
               \vspace{0pt}
               \begin{center}
               \tiny{\textbf{\textsf{\phantom{g}7\phantom{g}}}}\\
               \fbox{\includegraphics[width=1.0\linewidth]{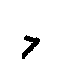}}
               \fbox{\includegraphics[width=1.0\linewidth]{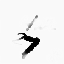}}
               \fbox{\includegraphics[width=1.0\linewidth]{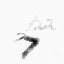}}
               \fbox{\includegraphics[width=1.0\linewidth]{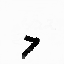}}
               \fbox{\includegraphics[width=1.0\linewidth]{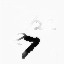}}
               \fbox{\includegraphics[width=1.0\linewidth]{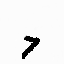}}
               \end{center}
            \end{minipage}
            \begin{minipage}[t]{0.09\linewidth}
               \vspace{0pt}
               \begin{center}
               \tiny{\textbf{\textsf{\phantom{g}8\phantom{g}}}}\\
               \fbox{\includegraphics[width=1.0\linewidth]{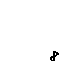}}
               \fbox{\includegraphics[width=1.0\linewidth]{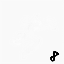}}
               \fbox{\includegraphics[width=1.0\linewidth]{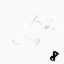}}
               \fbox{\includegraphics[width=1.0\linewidth]{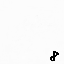}}
               \fbox{\includegraphics[width=1.0\linewidth]{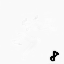}}
               \fbox{\includegraphics[width=1.0\linewidth]{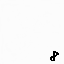}}
               \end{center}
            \end{minipage}
            \begin{minipage}[t]{0.09\linewidth}
               \vspace{0pt}
               \begin{center}
               \tiny{\textbf{\textsf{\phantom{g}9\phantom{g}}}}\\
               \fbox{\includegraphics[width=1.0\linewidth]{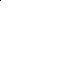}}
               \fbox{\includegraphics[width=1.0\linewidth]{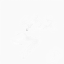}}
               \fbox{\includegraphics[width=1.0\linewidth]{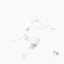}}
               \fbox{\includegraphics[width=1.0\linewidth]{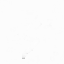}}
               \fbox{\includegraphics[width=1.0\linewidth]{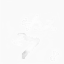}}
               \fbox{\includegraphics[width=1.0\linewidth]{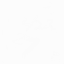}}
               \end{center}
            \end{minipage}
            \end{center}
         \end{minipage}
         % method labels
         \begin{minipage}[t]{0.04\linewidth}
            \vspace{0pt}
            \begin{rotate}{270}
               \tiny{\textbf{\textsf{
                  \hspace*{8pt}
                  True
                  \hspace*{4pt}
                  U-NET
                  \hspace*{7pt}
                  SG
                  \hspace*{8pt}
                  R-SG
                  \hspace*{6pt}
                  PMG
                  \hspace*{4pt}
                  R-PMG
               }}}
            \end{rotate}
         \end{minipage}
      \end{center}
   \end{minipage}
   \end{center}
\end{minipage}\\
\vspace{0.05\linewidth}
\begin{minipage}[t]{0.4975\linewidth}
   \vspace{0pt}
   % example 00229
   \begin{center}
   \begin{minipage}[t]{0.09\linewidth}
      \vspace{0pt}
      \begin{center}
         \tiny{\textbf{\textsf{Input}}}\\
         \fbox{\includegraphics[width=1.0\linewidth]{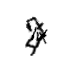}}
      \end{center}
   \end{minipage}
   \hfill
   \begin{minipage}[t]{0.90\linewidth}
      \vspace{0pt}
      \begin{center}
         % digits output
         \begin{minipage}[t]{0.94\linewidth}
            \vspace{0pt}
            \begin{center}
            \begin{minipage}[t]{0.09\linewidth}
               \vspace{0pt}
               \begin{center}
               \tiny{\textbf{\textsf{Digit: 0}}}\\
               \fbox{\includegraphics[width=1.0\linewidth]{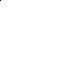}}
               \fbox{\includegraphics[width=1.0\linewidth]{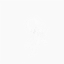}}
               \fbox{\includegraphics[width=1.0\linewidth]{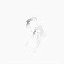}}
               \fbox{\includegraphics[width=1.0\linewidth]{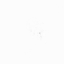}}
               \fbox{\includegraphics[width=1.0\linewidth]{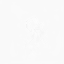}}
               \fbox{\includegraphics[width=1.0\linewidth]{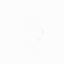}}
               \end{center}
            \end{minipage}
            \begin{minipage}[t]{0.09\linewidth}
               \vspace{0pt}
               \begin{center}
               \tiny{\textbf{\textsf{\phantom{g}1\phantom{g}}}}\\
               \fbox{\includegraphics[width=1.0\linewidth]{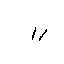}}
               \fbox{\includegraphics[width=1.0\linewidth]{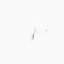}}
               \fbox{\includegraphics[width=1.0\linewidth]{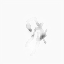}}
               \fbox{\includegraphics[width=1.0\linewidth]{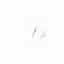}}
               \fbox{\includegraphics[width=1.0\linewidth]{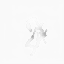}}
               \fbox{\includegraphics[width=1.0\linewidth]{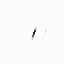}}
               \end{center}
            \end{minipage}
            \begin{minipage}[t]{0.09\linewidth}
               \vspace{0pt}
               \begin{center}
               \tiny{\textbf{\textsf{\phantom{g}2\phantom{g}}}}\\
               \fbox{\includegraphics[width=1.0\linewidth]{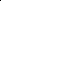}}
               \fbox{\includegraphics[width=1.0\linewidth]{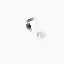}}
               \fbox{\includegraphics[width=1.0\linewidth]{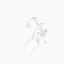}}
               \fbox{\includegraphics[width=1.0\linewidth]{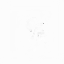}}
               \fbox{\includegraphics[width=1.0\linewidth]{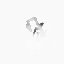}}
               \fbox{\includegraphics[width=1.0\linewidth]{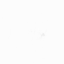}}
               \end{center}
            \end{minipage}
            \begin{minipage}[t]{0.09\linewidth}
               \vspace{0pt}
               \begin{center}
               \tiny{\textbf{\textsf{\phantom{g}3\phantom{g}}}}\\
               \fbox{\includegraphics[width=1.0\linewidth]{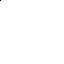}}
               \fbox{\includegraphics[width=1.0\linewidth]{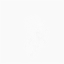}}
               \fbox{\includegraphics[width=1.0\linewidth]{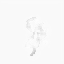}}
               \fbox{\includegraphics[width=1.0\linewidth]{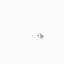}}
               \fbox{\includegraphics[width=1.0\linewidth]{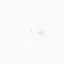}}
               \fbox{\includegraphics[width=1.0\linewidth]{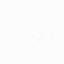}}
               \end{center}
            \end{minipage}
            \begin{minipage}[t]{0.09\linewidth}
               \vspace{0pt}
               \begin{center}
               \tiny{\textbf{\textsf{\phantom{g}4\phantom{g}}}}\\
               \fbox{\includegraphics[width=1.0\linewidth]{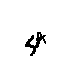}}
               \fbox{\includegraphics[width=1.0\linewidth]{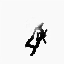}}
               \fbox{\includegraphics[width=1.0\linewidth]{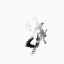}}
               \fbox{\includegraphics[width=1.0\linewidth]{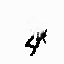}}
               \fbox{\includegraphics[width=1.0\linewidth]{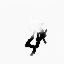}}
               \fbox{\includegraphics[width=1.0\linewidth]{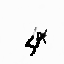}}
               \end{center}
            \end{minipage}
            \begin{minipage}[t]{0.09\linewidth}
               \vspace{0pt}
               \begin{center}
               \tiny{\textbf{\textsf{\phantom{g}5\phantom{g}}}}\\
               \fbox{\includegraphics[width=1.0\linewidth]{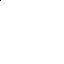}}
               \fbox{\includegraphics[width=1.0\linewidth]{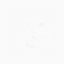}}
               \fbox{\includegraphics[width=1.0\linewidth]{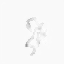}}
               \fbox{\includegraphics[width=1.0\linewidth]{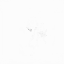}}
               \fbox{\includegraphics[width=1.0\linewidth]{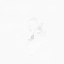}}
               \fbox{\includegraphics[width=1.0\linewidth]{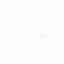}}
               \end{center}
            \end{minipage}
            \begin{minipage}[t]{0.09\linewidth}
               \vspace{0pt}
               \begin{center}
               \tiny{\textbf{\textsf{\phantom{g}6\phantom{g}}}}\\
               \fbox{\includegraphics[width=1.0\linewidth]{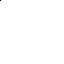}}
               \fbox{\includegraphics[width=1.0\linewidth]{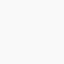}}
               \fbox{\includegraphics[width=1.0\linewidth]{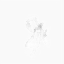}}
               \fbox{\includegraphics[width=1.0\linewidth]{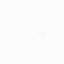}}
               \fbox{\includegraphics[width=1.0\linewidth]{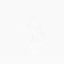}}
               \fbox{\includegraphics[width=1.0\linewidth]{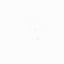}}
               \end{center}
            \end{minipage}
            \begin{minipage}[t]{0.09\linewidth}
               \vspace{0pt}
               \begin{center}
               \tiny{\textbf{\textsf{\phantom{g}7\phantom{g}}}}\\
               \fbox{\includegraphics[width=1.0\linewidth]{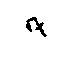}}
               \fbox{\includegraphics[width=1.0\linewidth]{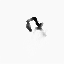}}
               \fbox{\includegraphics[width=1.0\linewidth]{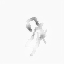}}
               \fbox{\includegraphics[width=1.0\linewidth]{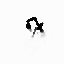}}
               \fbox{\includegraphics[width=1.0\linewidth]{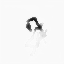}}
               \fbox{\includegraphics[width=1.0\linewidth]{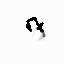}}
               \end{center}
            \end{minipage}
            \begin{minipage}[t]{0.09\linewidth}
               \vspace{0pt}
               \begin{center}
               \tiny{\textbf{\textsf{\phantom{g}8\phantom{g}}}}\\
               \fbox{\includegraphics[width=1.0\linewidth]{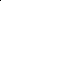}}
               \fbox{\includegraphics[width=1.0\linewidth]{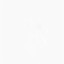}}
               \fbox{\includegraphics[width=1.0\linewidth]{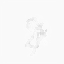}}
               \fbox{\includegraphics[width=1.0\linewidth]{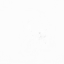}}
               \fbox{\includegraphics[width=1.0\linewidth]{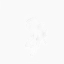}}
               \fbox{\includegraphics[width=1.0\linewidth]{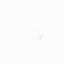}}
               \end{center}
            \end{minipage}
            \begin{minipage}[t]{0.09\linewidth}
               \vspace{0pt}
               \begin{center}
               \tiny{\textbf{\textsf{\phantom{g}9\phantom{g}}}}\\
               \fbox{\includegraphics[width=1.0\linewidth]{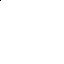}}
               \fbox{\includegraphics[width=1.0\linewidth]{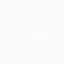}}
               \fbox{\includegraphics[width=1.0\linewidth]{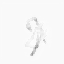}}
               \fbox{\includegraphics[width=1.0\linewidth]{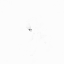}}
               \fbox{\includegraphics[width=1.0\linewidth]{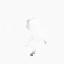}}
               \fbox{\includegraphics[width=1.0\linewidth]{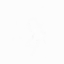}}
               \end{center}
            \end{minipage}
            \end{center}
         \end{minipage}
         % method labels
         \begin{minipage}[t]{0.04\linewidth}
            \vspace{0pt}
            \begin{rotate}{270}
               \tiny{\textbf{\textsf{
                  \hspace*{8pt}
                  True
                  \hspace*{4pt}
                  U-NET
                  \hspace*{7pt}
                  SG
                  \hspace*{8pt}
                  R-SG
                  \hspace*{6pt}
                  PMG
                  \hspace*{4pt}
                  R-PMG
               }}}
            \end{rotate}
         \end{minipage}
      \end{center}
   \end{minipage}
   \end{center}
\end{minipage}
\hfill
\begin{minipage}[t]{0.4975\linewidth}
   \vspace{0pt}
   % example 00240
   \begin{center}
   \begin{minipage}[t]{0.09\linewidth}
      \vspace{0pt}
      \begin{center}
         \tiny{\textbf{\textsf{Input}}}\\
         \fbox{\includegraphics[width=1.0\linewidth]{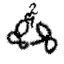}}
      \end{center}
   \end{minipage}
   \hfill
   \begin{minipage}[t]{0.90\linewidth}
      \vspace{0pt}
      \begin{center}
         % digits output
         \begin{minipage}[t]{0.94\linewidth}
            \vspace{0pt}
            \begin{center}
            \begin{minipage}[t]{0.09\linewidth}
               \vspace{0pt}
               \begin{center}
               \tiny{\textbf{\textsf{Digit: 0}}}\\
               \fbox{\includegraphics[width=1.0\linewidth]{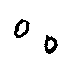}}
               \fbox{\includegraphics[width=1.0\linewidth]{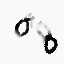}}
               \fbox{\includegraphics[width=1.0\linewidth]{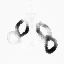}}
               \fbox{\includegraphics[width=1.0\linewidth]{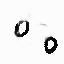}}
               \fbox{\includegraphics[width=1.0\linewidth]{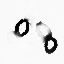}}
               \fbox{\includegraphics[width=1.0\linewidth]{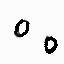}}
               \end{center}
            \end{minipage}
            \begin{minipage}[t]{0.09\linewidth}
               \vspace{0pt}
               \begin{center}
               \tiny{\textbf{\textsf{\phantom{g}1\phantom{g}}}}\\
               \fbox{\includegraphics[width=1.0\linewidth]{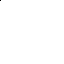}}
               \fbox{\includegraphics[width=1.0\linewidth]{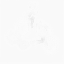}}
               \fbox{\includegraphics[width=1.0\linewidth]{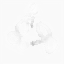}}
               \fbox{\includegraphics[width=1.0\linewidth]{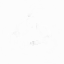}}
               \fbox{\includegraphics[width=1.0\linewidth]{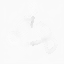}}
               \fbox{\includegraphics[width=1.0\linewidth]{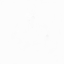}}
               \end{center}
            \end{minipage}
            \begin{minipage}[t]{0.09\linewidth}
               \vspace{0pt}
               \begin{center}
               \tiny{\textbf{\textsf{\phantom{g}2\phantom{g}}}}\\
               \fbox{\includegraphics[width=1.0\linewidth]{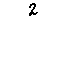}}
               \fbox{\includegraphics[width=1.0\linewidth]{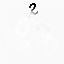}}
               \fbox{\includegraphics[width=1.0\linewidth]{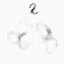}}
               \fbox{\includegraphics[width=1.0\linewidth]{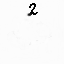}}
               \fbox{\includegraphics[width=1.0\linewidth]{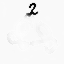}}
               \fbox{\includegraphics[width=1.0\linewidth]{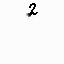}}
               \end{center}
            \end{minipage}
            \begin{minipage}[t]{0.09\linewidth}
               \vspace{0pt}
               \begin{center}
               \tiny{\textbf{\textsf{\phantom{g}3\phantom{g}}}}\\
               \fbox{\includegraphics[width=1.0\linewidth]{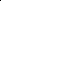}}
               \fbox{\includegraphics[width=1.0\linewidth]{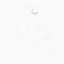}}
               \fbox{\includegraphics[width=1.0\linewidth]{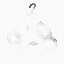}}
               \fbox{\includegraphics[width=1.0\linewidth]{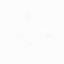}}
               \fbox{\includegraphics[width=1.0\linewidth]{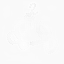}}
               \fbox{\includegraphics[width=1.0\linewidth]{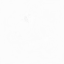}}
               \end{center}
            \end{minipage}
            \begin{minipage}[t]{0.09\linewidth}
               \vspace{0pt}
               \begin{center}
               \tiny{\textbf{\textsf{\phantom{g}4\phantom{g}}}}\\
               \fbox{\includegraphics[width=1.0\linewidth]{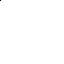}}
               \fbox{\includegraphics[width=1.0\linewidth]{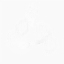}}
               \fbox{\includegraphics[width=1.0\linewidth]{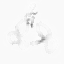}}
               \fbox{\includegraphics[width=1.0\linewidth]{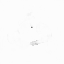}}
               \fbox{\includegraphics[width=1.0\linewidth]{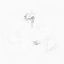}}
               \fbox{\includegraphics[width=1.0\linewidth]{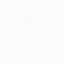}}
               \end{center}
            \end{minipage}
            \begin{minipage}[t]{0.09\linewidth}
               \vspace{0pt}
               \begin{center}
               \tiny{\textbf{\textsf{\phantom{g}5\phantom{g}}}}\\
               \fbox{\includegraphics[width=1.0\linewidth]{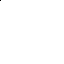}}
               \fbox{\includegraphics[width=1.0\linewidth]{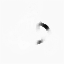}}
               \fbox{\includegraphics[width=1.0\linewidth]{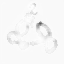}}
               \fbox{\includegraphics[width=1.0\linewidth]{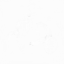}}
               \fbox{\includegraphics[width=1.0\linewidth]{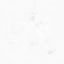}}
               \fbox{\includegraphics[width=1.0\linewidth]{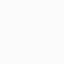}}
               \end{center}
            \end{minipage}
            \begin{minipage}[t]{0.09\linewidth}
               \vspace{0pt}
               \begin{center}
               \tiny{\textbf{\textsf{\phantom{g}6\phantom{g}}}}\\
               \fbox{\includegraphics[width=1.0\linewidth]{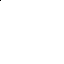}}
               \fbox{\includegraphics[width=1.0\linewidth]{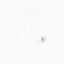}}
               \fbox{\includegraphics[width=1.0\linewidth]{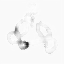}}
               \fbox{\includegraphics[width=1.0\linewidth]{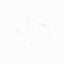}}
               \fbox{\includegraphics[width=1.0\linewidth]{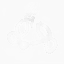}}
               \fbox{\includegraphics[width=1.0\linewidth]{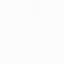}}
               \end{center}
            \end{minipage}
            \begin{minipage}[t]{0.09\linewidth}
               \vspace{0pt}
               \begin{center}
               \tiny{\textbf{\textsf{\phantom{g}7\phantom{g}}}}\\
               \fbox{\includegraphics[width=1.0\linewidth]{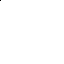}}
               \fbox{\includegraphics[width=1.0\linewidth]{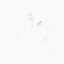}}
               \fbox{\includegraphics[width=1.0\linewidth]{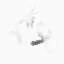}}
               \fbox{\includegraphics[width=1.0\linewidth]{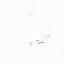}}
               \fbox{\includegraphics[width=1.0\linewidth]{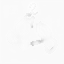}}
               \fbox{\includegraphics[width=1.0\linewidth]{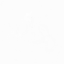}}
               \end{center}
            \end{minipage}
            \begin{minipage}[t]{0.09\linewidth}
               \vspace{0pt}
               \begin{center}
               \tiny{\textbf{\textsf{\phantom{g}8\phantom{g}}}}\\
               \fbox{\includegraphics[width=1.0\linewidth]{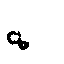}}
               \fbox{\includegraphics[width=1.0\linewidth]{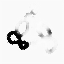}}
               \fbox{\includegraphics[width=1.0\linewidth]{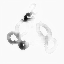}}
               \fbox{\includegraphics[width=1.0\linewidth]{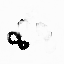}}
               \fbox{\includegraphics[width=1.0\linewidth]{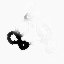}}
               \fbox{\includegraphics[width=1.0\linewidth]{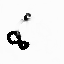}}
               \end{center}
            \end{minipage}
            \begin{minipage}[t]{0.09\linewidth}
               \vspace{0pt}
               \begin{center}
               \tiny{\textbf{\textsf{\phantom{g}9\phantom{g}}}}\\
               \fbox{\includegraphics[width=1.0\linewidth]{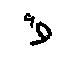}}
               \fbox{\includegraphics[width=1.0\linewidth]{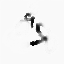}}
               \fbox{\includegraphics[width=1.0\linewidth]{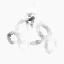}}
               \fbox{\includegraphics[width=1.0\linewidth]{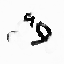}}
               \fbox{\includegraphics[width=1.0\linewidth]{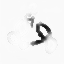}}
               \fbox{\includegraphics[width=1.0\linewidth]{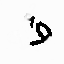}}
               \end{center}
            \end{minipage}
            \end{center}
         \end{minipage}
         % method labels
         \begin{minipage}[t]{0.04\linewidth}
            \vspace{0pt}
            \begin{rotate}{270}
               \tiny{\textbf{\textsf{
                  \hspace*{8pt}
                  True
                  \hspace*{4pt}
                  U-NET
                  \hspace*{7pt}
                  SG
                  \hspace*{8pt}
                  R-SG
                  \hspace*{6pt}
                  PMG
                  \hspace*{4pt}
                  R-PMG
               }}}
            \end{rotate}
         \end{minipage}
      \end{center}
   \end{minipage}
   \end{center}
\end{minipage}\\
\vspace{0.05\linewidth}
\begin{minipage}[t]{0.4975\linewidth}
   \vspace{0pt}
   % example 00269
   \begin{center}
   \begin{minipage}[t]{0.09\linewidth}
      \vspace{0pt}
      \begin{center}
         \tiny{\textbf{\textsf{Input}}}\\
         \fbox{\includegraphics[width=1.0\linewidth]{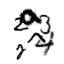}}
      \end{center}
   \end{minipage}
   \hfill
   \begin{minipage}[t]{0.90\linewidth}
      \vspace{0pt}
      \begin{center}
         % digits output
         \begin{minipage}[t]{0.94\linewidth}
            \vspace{0pt}
            \begin{center}
            \begin{minipage}[t]{0.09\linewidth}
               \vspace{0pt}
               \begin{center}
               \tiny{\textbf{\textsf{Digit: 0}}}\\
               \fbox{\includegraphics[width=1.0\linewidth]{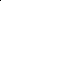}}
               \fbox{\includegraphics[width=1.0\linewidth]{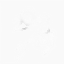}}
               \fbox{\includegraphics[width=1.0\linewidth]{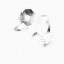}}
               \fbox{\includegraphics[width=1.0\linewidth]{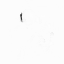}}
               \fbox{\includegraphics[width=1.0\linewidth]{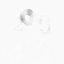}}
               \fbox{\includegraphics[width=1.0\linewidth]{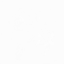}}
               \end{center}
            \end{minipage}
            \begin{minipage}[t]{0.09\linewidth}
               \vspace{0pt}
               \begin{center}
               \tiny{\textbf{\textsf{\phantom{g}1\phantom{g}}}}\\
               \fbox{\includegraphics[width=1.0\linewidth]{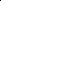}}
               \fbox{\includegraphics[width=1.0\linewidth]{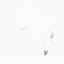}}
               \fbox{\includegraphics[width=1.0\linewidth]{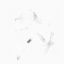}}
               \fbox{\includegraphics[width=1.0\linewidth]{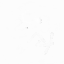}}
               \fbox{\includegraphics[width=1.0\linewidth]{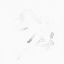}}
               \fbox{\includegraphics[width=1.0\linewidth]{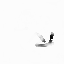}}
               \end{center}
            \end{minipage}
            \begin{minipage}[t]{0.09\linewidth}
               \vspace{0pt}
               \begin{center}
               \tiny{\textbf{\textsf{\phantom{g}2\phantom{g}}}}\\
               \fbox{\includegraphics[width=1.0\linewidth]{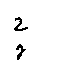}}
               \fbox{\includegraphics[width=1.0\linewidth]{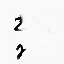}}
               \fbox{\includegraphics[width=1.0\linewidth]{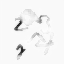}}
               \fbox{\includegraphics[width=1.0\linewidth]{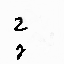}}
               \fbox{\includegraphics[width=1.0\linewidth]{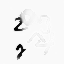}}
               \fbox{\includegraphics[width=1.0\linewidth]{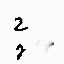}}
               \end{center}
            \end{minipage}
            \begin{minipage}[t]{0.09\linewidth}
               \vspace{0pt}
               \begin{center}
               \tiny{\textbf{\textsf{\phantom{g}3\phantom{g}}}}\\
               \fbox{\includegraphics[width=1.0\linewidth]{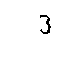}}
               \fbox{\includegraphics[width=1.0\linewidth]{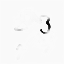}}
               \fbox{\includegraphics[width=1.0\linewidth]{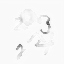}}
               \fbox{\includegraphics[width=1.0\linewidth]{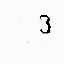}}
               \fbox{\includegraphics[width=1.0\linewidth]{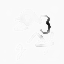}}
               \fbox{\includegraphics[width=1.0\linewidth]{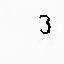}}
               \end{center}
            \end{minipage}
            \begin{minipage}[t]{0.09\linewidth}
               \vspace{0pt}
               \begin{center}
               \tiny{\textbf{\textsf{\phantom{g}4\phantom{g}}}}\\
               \fbox{\includegraphics[width=1.0\linewidth]{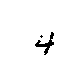}}
               \fbox{\includegraphics[width=1.0\linewidth]{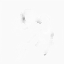}}
               \fbox{\includegraphics[width=1.0\linewidth]{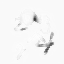}}
               \fbox{\includegraphics[width=1.0\linewidth]{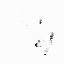}}
               \fbox{\includegraphics[width=1.0\linewidth]{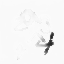}}
               \fbox{\includegraphics[width=1.0\linewidth]{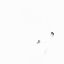}}
               \end{center}
            \end{minipage}
            \begin{minipage}[t]{0.09\linewidth}
               \vspace{0pt}
               \begin{center}
               \tiny{\textbf{\textsf{\phantom{g}5\phantom{g}}}}\\
               \fbox{\includegraphics[width=1.0\linewidth]{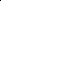}}
               \fbox{\includegraphics[width=1.0\linewidth]{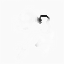}}
               \fbox{\includegraphics[width=1.0\linewidth]{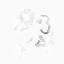}}
               \fbox{\includegraphics[width=1.0\linewidth]{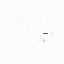}}
               \fbox{\includegraphics[width=1.0\linewidth]{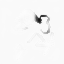}}
               \fbox{\includegraphics[width=1.0\linewidth]{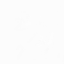}}
               \end{center}
            \end{minipage}
            \begin{minipage}[t]{0.09\linewidth}
               \vspace{0pt}
               \begin{center}
               \tiny{\textbf{\textsf{\phantom{g}6\phantom{g}}}}\\
               \fbox{\includegraphics[width=1.0\linewidth]{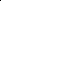}}
               \fbox{\includegraphics[width=1.0\linewidth]{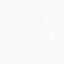}}
               \fbox{\includegraphics[width=1.0\linewidth]{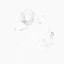}}
               \fbox{\includegraphics[width=1.0\linewidth]{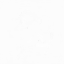}}
               \fbox{\includegraphics[width=1.0\linewidth]{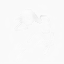}}
               \fbox{\includegraphics[width=1.0\linewidth]{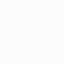}}
               \end{center}
            \end{minipage}
            \begin{minipage}[t]{0.09\linewidth}
               \vspace{0pt}
               \begin{center}
               \tiny{\textbf{\textsf{\phantom{g}7\phantom{g}}}}\\
               \fbox{\includegraphics[width=1.0\linewidth]{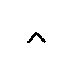}}
               \fbox{\includegraphics[width=1.0\linewidth]{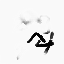}}
               \fbox{\includegraphics[width=1.0\linewidth]{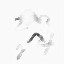}}
               \fbox{\includegraphics[width=1.0\linewidth]{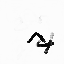}}
               \fbox{\includegraphics[width=1.0\linewidth]{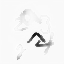}}
               \fbox{\includegraphics[width=1.0\linewidth]{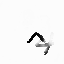}}
               \end{center}
            \end{minipage}
            \begin{minipage}[t]{0.09\linewidth}
               \vspace{0pt}
               \begin{center}
               \tiny{\textbf{\textsf{\phantom{g}8\phantom{g}}}}\\
               \fbox{\includegraphics[width=1.0\linewidth]{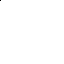}}
               \fbox{\includegraphics[width=1.0\linewidth]{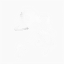}}
               \fbox{\includegraphics[width=1.0\linewidth]{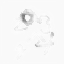}}
               \fbox{\includegraphics[width=1.0\linewidth]{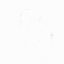}}
               \fbox{\includegraphics[width=1.0\linewidth]{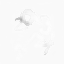}}
               \fbox{\includegraphics[width=1.0\linewidth]{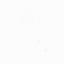}}
               \end{center}
            \end{minipage}
            \begin{minipage}[t]{0.09\linewidth}
               \vspace{0pt}
               \begin{center}
               \tiny{\textbf{\textsf{\phantom{g}9\phantom{g}}}}\\
               \fbox{\includegraphics[width=1.0\linewidth]{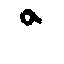}}
               \fbox{\includegraphics[width=1.0\linewidth]{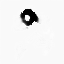}}
               \fbox{\includegraphics[width=1.0\linewidth]{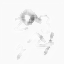}}
               \fbox{\includegraphics[width=1.0\linewidth]{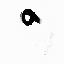}}
               \fbox{\includegraphics[width=1.0\linewidth]{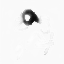}}
               \fbox{\includegraphics[width=1.0\linewidth]{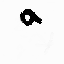}}
               \end{center}
            \end{minipage}
            \end{center}
         \end{minipage}
         % method labels
         \begin{minipage}[t]{0.04\linewidth}
            \vspace{0pt}
            \begin{rotate}{270}
               \tiny{\textbf{\textsf{
                  \hspace*{8pt}
                  True
                  \hspace*{4pt}
                  U-NET
                  \hspace*{7pt}
                  SG
                  \hspace*{8pt}
                  R-SG
                  \hspace*{6pt}
                  PMG
                  \hspace*{4pt}
                  R-PMG
               }}}
            \end{rotate}
         \end{minipage}
      \end{center}
   \end{minipage}
   \end{center}
\end{minipage}
\hfill
\begin{minipage}[t]{0.4975\linewidth}
   \vspace{0pt}
   % example 00304
   \begin{center}
   \begin{minipage}[t]{0.09\linewidth}
      \vspace{0pt}
      \begin{center}
         \tiny{\textbf{\textsf{Input}}}\\
         \fbox{\includegraphics[width=1.0\linewidth]{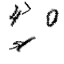}}
      \end{center}
   \end{minipage}
   \hfill
   \begin{minipage}[t]{0.90\linewidth}
      \vspace{0pt}
      \begin{center}
         % digits output
         \begin{minipage}[t]{0.94\linewidth}
            \vspace{0pt}
            \begin{center}
            \begin{minipage}[t]{0.09\linewidth}
               \vspace{0pt}
               \begin{center}
               \tiny{\textbf{\textsf{Digit: 0}}}\\
               \fbox{\includegraphics[width=1.0\linewidth]{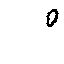}}
               \fbox{\includegraphics[width=1.0\linewidth]{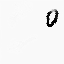}}
               \fbox{\includegraphics[width=1.0\linewidth]{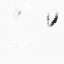}}
               \fbox{\includegraphics[width=1.0\linewidth]{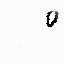}}
               \fbox{\includegraphics[width=1.0\linewidth]{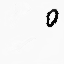}}
               \fbox{\includegraphics[width=1.0\linewidth]{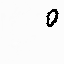}}
               \end{center}
            \end{minipage}
            \begin{minipage}[t]{0.09\linewidth}
               \vspace{0pt}
               \begin{center}
               \tiny{\textbf{\textsf{\phantom{g}1\phantom{g}}}}\\
               \fbox{\includegraphics[width=1.0\linewidth]{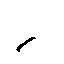}}
               \fbox{\includegraphics[width=1.0\linewidth]{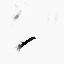}}
               \fbox{\includegraphics[width=1.0\linewidth]{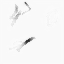}}
               \fbox{\includegraphics[width=1.0\linewidth]{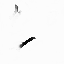}}
               \fbox{\includegraphics[width=1.0\linewidth]{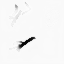}}
               \fbox{\includegraphics[width=1.0\linewidth]{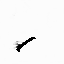}}
               \end{center}
            \end{minipage}
            \begin{minipage}[t]{0.09\linewidth}
               \vspace{0pt}
               \begin{center}
               \tiny{\textbf{\textsf{\phantom{g}2\phantom{g}}}}\\
               \fbox{\includegraphics[width=1.0\linewidth]{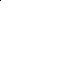}}
               \fbox{\includegraphics[width=1.0\linewidth]{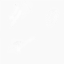}}
               \fbox{\includegraphics[width=1.0\linewidth]{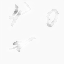}}
               \fbox{\includegraphics[width=1.0\linewidth]{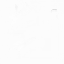}}
               \fbox{\includegraphics[width=1.0\linewidth]{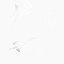}}
               \fbox{\includegraphics[width=1.0\linewidth]{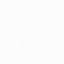}}
               \end{center}
            \end{minipage}
            \begin{minipage}[t]{0.09\linewidth}
               \vspace{0pt}
               \begin{center}
               \tiny{\textbf{\textsf{\phantom{g}3\phantom{g}}}}\\
               \fbox{\includegraphics[width=1.0\linewidth]{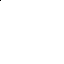}}
               \fbox{\includegraphics[width=1.0\linewidth]{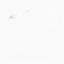}}
               \fbox{\includegraphics[width=1.0\linewidth]{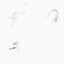}}
               \fbox{\includegraphics[width=1.0\linewidth]{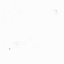}}
               \fbox{\includegraphics[width=1.0\linewidth]{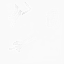}}
               \fbox{\includegraphics[width=1.0\linewidth]{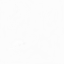}}
               \end{center}
            \end{minipage}
            \begin{minipage}[t]{0.09\linewidth}
               \vspace{0pt}
               \begin{center}
               \tiny{\textbf{\textsf{\phantom{g}4\phantom{g}}}}\\
               \fbox{\includegraphics[width=1.0\linewidth]{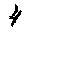}}
               \fbox{\includegraphics[width=1.0\linewidth]{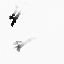}}
               \fbox{\includegraphics[width=1.0\linewidth]{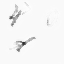}}
               \fbox{\includegraphics[width=1.0\linewidth]{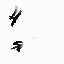}}
               \fbox{\includegraphics[width=1.0\linewidth]{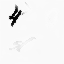}}
               \fbox{\includegraphics[width=1.0\linewidth]{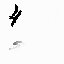}}
               \end{center}
            \end{minipage}
            \begin{minipage}[t]{0.09\linewidth}
               \vspace{0pt}
               \begin{center}
               \tiny{\textbf{\textsf{\phantom{g}5\phantom{g}}}}\\
               \fbox{\includegraphics[width=1.0\linewidth]{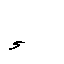}}
               \fbox{\includegraphics[width=1.0\linewidth]{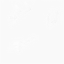}}
               \fbox{\includegraphics[width=1.0\linewidth]{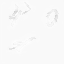}}
               \fbox{\includegraphics[width=1.0\linewidth]{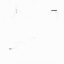}}
               \fbox{\includegraphics[width=1.0\linewidth]{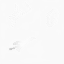}}
               \fbox{\includegraphics[width=1.0\linewidth]{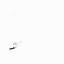}}
               \end{center}
            \end{minipage}
            \begin{minipage}[t]{0.09\linewidth}
               \vspace{0pt}
               \begin{center}
               \tiny{\textbf{\textsf{\phantom{g}6\phantom{g}}}}\\
               \fbox{\includegraphics[width=1.0\linewidth]{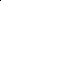}}
               \fbox{\includegraphics[width=1.0\linewidth]{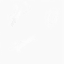}}
               \fbox{\includegraphics[width=1.0\linewidth]{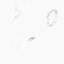}}
               \fbox{\includegraphics[width=1.0\linewidth]{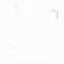}}
               \fbox{\includegraphics[width=1.0\linewidth]{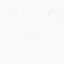}}
               \fbox{\includegraphics[width=1.0\linewidth]{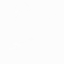}}
               \end{center}
            \end{minipage}
            \begin{minipage}[t]{0.09\linewidth}
               \vspace{0pt}
               \begin{center}
               \tiny{\textbf{\textsf{\phantom{g}7\phantom{g}}}}\\
               \fbox{\includegraphics[width=1.0\linewidth]{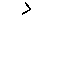}}
               \fbox{\includegraphics[width=1.0\linewidth]{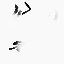}}
               \fbox{\includegraphics[width=1.0\linewidth]{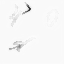}}
               \fbox{\includegraphics[width=1.0\linewidth]{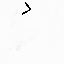}}
               \fbox{\includegraphics[width=1.0\linewidth]{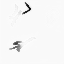}}
               \fbox{\includegraphics[width=1.0\linewidth]{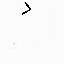}}
               \end{center}
            \end{minipage}
            \begin{minipage}[t]{0.09\linewidth}
               \vspace{0pt}
               \begin{center}
               \tiny{\textbf{\textsf{\phantom{g}8\phantom{g}}}}\\
               \fbox{\includegraphics[width=1.0\linewidth]{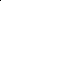}}
               \fbox{\includegraphics[width=1.0\linewidth]{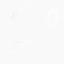}}
               \fbox{\includegraphics[width=1.0\linewidth]{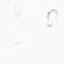}}
               \fbox{\includegraphics[width=1.0\linewidth]{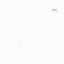}}
               \fbox{\includegraphics[width=1.0\linewidth]{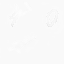}}
               \fbox{\includegraphics[width=1.0\linewidth]{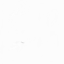}}
               \end{center}
            \end{minipage}
            \begin{minipage}[t]{0.09\linewidth}
               \vspace{0pt}
               \begin{center}
               \tiny{\textbf{\textsf{\phantom{g}9\phantom{g}}}}\\
               \fbox{\includegraphics[width=1.0\linewidth]{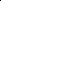}}
               \fbox{\includegraphics[width=1.0\linewidth]{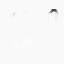}}
               \fbox{\includegraphics[width=1.0\linewidth]{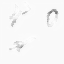}}
               \fbox{\includegraphics[width=1.0\linewidth]{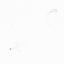}}
               \fbox{\includegraphics[width=1.0\linewidth]{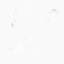}}
               \fbox{\includegraphics[width=1.0\linewidth]{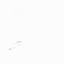}}
               \end{center}
            \end{minipage}
            \end{center}
         \end{minipage}
         % method labels
         \begin{minipage}[t]{0.04\linewidth}
            \vspace{0pt}
            \begin{rotate}{270}
               \tiny{\textbf{\textsf{
                  \hspace*{8pt}
                  True
                  \hspace*{4pt}
                  U-NET
                  \hspace*{7pt}
                  SG
                  \hspace*{8pt}
                  R-SG
                  \hspace*{6pt}
                  PMG
                  \hspace*{4pt}
                  R-PMG
               }}}
            \end{rotate}
         \end{minipage}
      \end{center}
   \end{minipage}
   \end{center}
\end{minipage}
