# Supplementary material for: Multigrid Neural Architectures
Source: arXiv:1611.07661 source file (2017-05-11)
Supplement: Supplementary file 2 [file fig_supp_spt_content.tex]

\setlength\fboxsep{0pt}
% spatial transform examples
\begin{minipage}[t]{1.00\linewidth}
   \vspace{0pt}
   \begin{center}
   \begin{minipage}[t]{0.13143\linewidth}
      \vspace{0pt}
      \begin{center}
      \tiny{\textbf{\textsf{Input}}}\\
      \fbox{\includegraphics[width=1.0\linewidth]{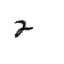}}
      \fbox{\includegraphics[width=1.0\linewidth]{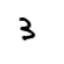}}
      \fbox{\includegraphics[width=1.0\linewidth]{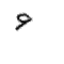}}
      \fbox{\includegraphics[width=1.0\linewidth]{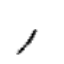}}
      \fbox{\includegraphics[width=1.0\linewidth]{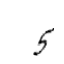}}
      \fbox{\includegraphics[width=1.0\linewidth]{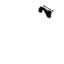}}
      \fbox{\includegraphics[width=1.0\linewidth]{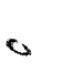}}
      \fbox{\includegraphics[width=1.0\linewidth]{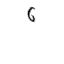}}
      \fbox{\includegraphics[width=1.0\linewidth]{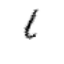}}
      \fbox{\includegraphics[width=1.0\linewidth]{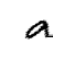}}
      \fbox{\includegraphics[width=1.0\linewidth]{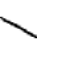}}
      \fbox{\includegraphics[width=1.0\linewidth]{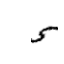}}
      \fbox{\includegraphics[width=1.0\linewidth]{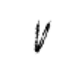}}
      \fbox{\includegraphics[width=1.0\linewidth]{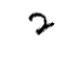}}
      %\fbox{\includegraphics[width=1.0\linewidth]{figures/mnist-spt/00114_input_1.png}}
      %\fbox{\includegraphics[width=1.0\linewidth]{figures/mnist-spt/00115_input_6.png}}
      \end{center}
   \end{minipage}
   \begin{minipage}[t]{0.13143\linewidth}
      \vspace{0pt}
      \begin{center}
      \tiny{\textbf{\textsf{\phantom{p}True\phantom{p}}}}\\
      \fbox{\includegraphics[width=1.0\linewidth]{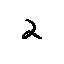}}
      \fbox{\includegraphics[width=1.0\linewidth]{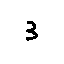}}
      \fbox{\includegraphics[width=1.0\linewidth]{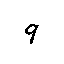}}
      \fbox{\includegraphics[width=1.0\linewidth]{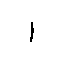}}
      \fbox{\includegraphics[width=1.0\linewidth]{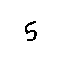}}
      \fbox{\includegraphics[width=1.0\linewidth]{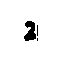}}
      \fbox{\includegraphics[width=1.0\linewidth]{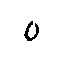}}
      \fbox{\includegraphics[width=1.0\linewidth]{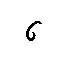}}
      \fbox{\includegraphics[width=1.0\linewidth]{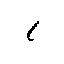}}
      \fbox{\includegraphics[width=1.0\linewidth]{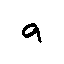}}
      \fbox{\includegraphics[width=1.0\linewidth]{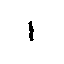}}
      \fbox{\includegraphics[width=1.0\linewidth]{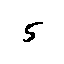}}
      \fbox{\includegraphics[width=1.0\linewidth]{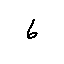}}
      \fbox{\includegraphics[width=1.0\linewidth]{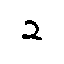}}
      %\fbox{\includegraphics[width=1.0\linewidth]{figures/mnist-spt/00114_label_1.png}}
      %\fbox{\includegraphics[width=1.0\linewidth]{figures/mnist-spt/00115_label_6.png}}
      \end{center}
   \end{minipage}
   \begin{minipage}[t]{0.13143\linewidth}
      \vspace{0pt}
      \begin{center}
      \tiny{\textbf{\textsf{\phantom{p}U-NET\phantom{p}}}}\\
      \fbox{\includegraphics[width=1.0\linewidth]{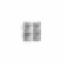}}
      \fbox{\includegraphics[width=1.0\linewidth]{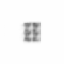}}
      \fbox{\includegraphics[width=1.0\linewidth]{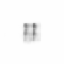}}
      \fbox{\includegraphics[width=1.0\linewidth]{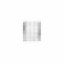}}
      \fbox{\includegraphics[width=1.0\linewidth]{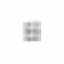}}
      \fbox{\includegraphics[width=1.0\linewidth]{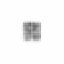}}
      \fbox{\includegraphics[width=1.0\linewidth]{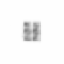}}
      \fbox{\includegraphics[width=1.0\linewidth]{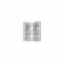}}
      \fbox{\includegraphics[width=1.0\linewidth]{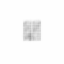}}
      \fbox{\includegraphics[width=1.0\linewidth]{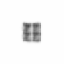}}
      \fbox{\includegraphics[width=1.0\linewidth]{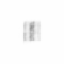}}
      \fbox{\includegraphics[width=1.0\linewidth]{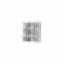}}
      \fbox{\includegraphics[width=1.0\linewidth]{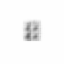}}
      \fbox{\includegraphics[width=1.0\linewidth]{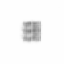}}
      %\fbox{\includegraphics[width=1.0\linewidth]{figures/mnist-spt/00114_unet_1.png}}
      %\fbox{\includegraphics[width=1.0\linewidth]{figures/mnist-spt/00115_unet_6.png}}
      \end{center}
   \end{minipage}
   \begin{minipage}[t]{0.13143\linewidth}
      \vspace{0pt}
      \begin{center}
      \tiny{\textbf{\textsf{\phantom{p}SG}\phantom{p}}}\\
      \fbox{\includegraphics[width=1.0\linewidth]{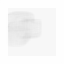}}
      \fbox{\includegraphics[width=1.0\linewidth]{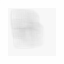}}
      \fbox{\includegraphics[width=1.0\linewidth]{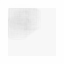}}
      \fbox{\includegraphics[width=1.0\linewidth]{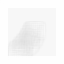}}
      \fbox{\includegraphics[width=1.0\linewidth]{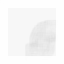}}
      \fbox{\includegraphics[width=1.0\linewidth]{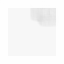}}
      \fbox{\includegraphics[width=1.0\linewidth]{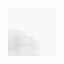}}
      \fbox{\includegraphics[width=1.0\linewidth]{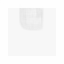}}
      \fbox{\includegraphics[width=1.0\linewidth]{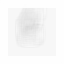}}
      \fbox{\includegraphics[width=1.0\linewidth]{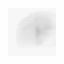}}
      \fbox{\includegraphics[width=1.0\linewidth]{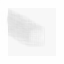}}
      \fbox{\includegraphics[width=1.0\linewidth]{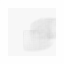}}
      \fbox{\includegraphics[width=1.0\linewidth]{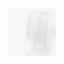}}
      \fbox{\includegraphics[width=1.0\linewidth]{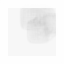}}
      %\fbox{\includegraphics[width=1.0\linewidth]{figures/mnist-spt/00114_pnmgsg_1.png}}
      %\fbox{\includegraphics[width=1.0\linewidth]{figures/mnist-spt/00115_pnmgsg_6.png}}
      \end{center}
   \end{minipage}
   \begin{minipage}[t]{0.13143\linewidth}
      \vspace{0pt}
      \begin{center}
      \tiny{\textbf{\textsf{\phantom{p}R-SG\phantom{p}}}}\\
      \fbox{\includegraphics[width=1.0\linewidth]{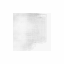}}
      \fbox{\includegraphics[width=1.0\linewidth]{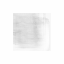}}
      \fbox{\includegraphics[width=1.0\linewidth]{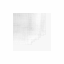}}
      \fbox{\includegraphics[width=1.0\linewidth]{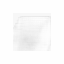}}
      \fbox{\includegraphics[width=1.0\linewidth]{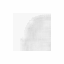}}
      \fbox{\includegraphics[width=1.0\linewidth]{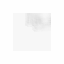}}
      \fbox{\includegraphics[width=1.0\linewidth]{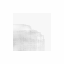}}
      \fbox{\includegraphics[width=1.0\linewidth]{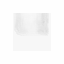}}
      \fbox{\includegraphics[width=1.0\linewidth]{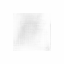}}
      \fbox{\includegraphics[width=1.0\linewidth]{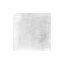}}
      \fbox{\includegraphics[width=1.0\linewidth]{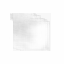}}
      \fbox{\includegraphics[width=1.0\linewidth]{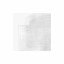}}
      \fbox{\includegraphics[width=1.0\linewidth]{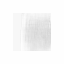}}
      \fbox{\includegraphics[width=1.0\linewidth]{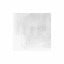}}
      %\fbox{\includegraphics[width=1.0\linewidth]{figures/mnist-spt/00114_prnmgsg_1.png}}
      %\fbox{\includegraphics[width=1.0\linewidth]{figures/mnist-spt/00115_prnmgsg_6.png}}
      \end{center}
   \end{minipage}
   \begin{minipage}[t]{0.13143\linewidth}
      \vspace{0pt}
      \begin{center}
      \tiny{\textbf{\textsf{\phantom{p}PMG\phantom{p}}}}\\
      \fbox{\includegraphics[width=1.0\linewidth]{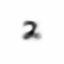}}
      \fbox{\includegraphics[width=1.0\linewidth]{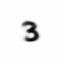}}
      \fbox{\includegraphics[width=1.0\linewidth]{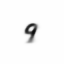}}
      \fbox{\includegraphics[width=1.0\linewidth]{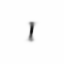}}
      \fbox{\includegraphics[width=1.0\linewidth]{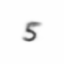}}
      \fbox{\includegraphics[width=1.0\linewidth]{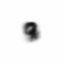}}
      \fbox{\includegraphics[width=1.0\linewidth]{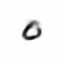}}
      \fbox{\includegraphics[width=1.0\linewidth]{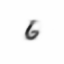}}
      \fbox{\includegraphics[width=1.0\linewidth]{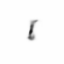}}
      \fbox{\includegraphics[width=1.0\linewidth]{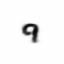}}
      \fbox{\includegraphics[width=1.0\linewidth]{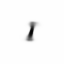}}
      \fbox{\includegraphics[width=1.0\linewidth]{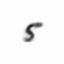}}
      \fbox{\includegraphics[width=1.0\linewidth]{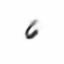}}
      \fbox{\includegraphics[width=1.0\linewidth]{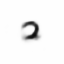}}
      %\fbox{\includegraphics[width=1.0\linewidth]{figures/mnist-spt/00114_pnmg2_1.png}}
      %\fbox{\includegraphics[width=1.0\linewidth]{figures/mnist-spt/00115_pnmg2_6.png}}
      \end{center}
   \end{minipage}
   \begin{minipage}[t]{0.13143\linewidth}
      \vspace{0pt}
      \begin{center}
      \tiny{\textbf{\textsf{\phantom{p}R-PMG\phantom{p}}}}\\
      \fbox{\includegraphics[width=1.0\linewidth]{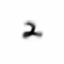}}
      \fbox{\includegraphics[width=1.0\linewidth]{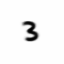}}
      \fbox{\includegraphics[width=1.0\linewidth]{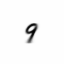}}
      \fbox{\includegraphics[width=1.0\linewidth]{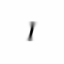}}
      \fbox{\includegraphics[width=1.0\linewidth]{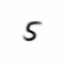}}
      \fbox{\includegraphics[width=1.0\linewidth]{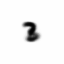}}
      \fbox{\includegraphics[width=1.0\linewidth]{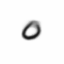}}
      \fbox{\includegraphics[width=1.0\linewidth]{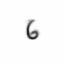}}
      \fbox{\includegraphics[width=1.0\linewidth]{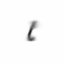}}
      \fbox{\includegraphics[width=1.0\linewidth]{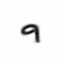}}
      \fbox{\includegraphics[width=1.0\linewidth]{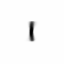}}
      \fbox{\includegraphics[width=1.0\linewidth]{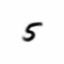}}
      \fbox{\includegraphics[width=1.0\linewidth]{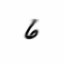}}
      \fbox{\includegraphics[width=1.0\linewidth]{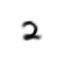}}
      %\fbox{\includegraphics[width=1.0\linewidth]{figures/mnist-spt/00114_prnmg2_1.png}}
      %\fbox{\includegraphics[width=1.0\linewidth]{figures/mnist-spt/00115_prnmg2_6.png}}
      \end{center}
   \end{minipage}\\
   \vspace{0.012\linewidth}
   \end{center}
\end{minipage}
